# Supplementary material for: Mesoscopic heterogeneity in biomolecular condensates from sequence patterning
Source: arXiv:2502.14587 ancillary file (2025-02-20)
Supplement: Supplementary file 1 [file supp.pdf]

## Supporting Information Text

### 1. Parameter-free grouping and clustering algorithm for the multi-polymer simulations

Here, we describe how we determine clusters and groups in the MD simulations that, in turn, determines the quantitative criteria for the multi-polymer phase diagrams. We define a cluster  $C^{(i)}(t)$ ,  $i = 1, \dots, N_C$  with  $N_C$  being the total number of clusters at time  $t$ , to be a collection of cohesive/opposite charged particles (list of particle indices) whose centers are vertices of at least one discrete path (or walk) with individual step lengths not exceeding the cohesive/charged interaction range  $r_{\text{coh/cha}}$ . In graph theoretical terms: a cluster is a connected graph where edges between nodes, nodes representing particle indices, are placed based upon a Euclidean distance criterion. No tuning/fitting parameters are required for the clustering procedure because the sole parameter that determines the clustering is a physical parameter of the already determine model. The cluster size,  $|C^{(i)}(t)|$ , has a range of  $1 \leq |C^{(i)}(t)| \leq N_{\text{coh}}$  for the cohesive-spacer polymers and  $1 \leq |C^{(i)}(t)| \leq N_{\text{cha}}/2$  for the charged-spacer polymers, where  $N_{\text{coh}}$  and  $N_{\text{cha}}$  are, respectively, the total number of cohesive beads and charged beads in the system. The lower bound is 1 as we count separated-individual beads as a single cluster. A cluster of maximum size is the largest mono-cluster.

We next describe how the clustering works in practice, focusing on the charged beads (as the cohesive case is simpler). At some prescribed time  $t$ , compute the distance  $r_{ij}$  for  $i \in \{1, \dots, N_{\text{cha}}\}$  and  $j \geq i$ , given  $i$  and  $j$  are opposite charges. If  $r_{ij} \leq r_{\text{cha}}$ , where  $r_{\text{cha}}$  is the range of the charged interaction, then  $i$  and  $j$  are in the same cluster. During the running of the algorithm, if two charged beads  $i$  and  $j$ , that are within  $r_{\text{cha}}$  of each other, have not yet been classified into a cluster then a new cluster  $C^{(k=N_C+1)} = (i, j)$  ( $N_C$  being the running total number of clusters) is created, if  $i$  does not already belong to a cluster  $i$  joins the cluster of  $j$ , likewise, if  $j$  does not already belong to a cluster  $j$  joins the cluster  $i$  belongs to. A final step is to coalesce clusters, *i.e.*, merge clusters that have particle indices in common.

Finally, we define a group  $G^{(i)}(t)$ ,  $i = 1, \dots, N_G$  with  $N_G$  being the total number of groups at time  $t$ , to be a collection of cluster indices determined through polymer connectivity. That is, if two clusters, say  $C^{(j)}$  and  $C^{(k)}$  each contain at least one bead from the same polymer then those two clusters form a group. As with the agglomeration of clusters, groups are merged with polymers in common. Polymers on their own can form a group.

### 2. Classification conditionals for the phase diagrams

**A. Cohesive-spacer polymers.** The following conditionals should be followed (executed) one-by-one in order to reproduce the phase diagram (see Figs. S3A and 2C):

1. “Polymer-gas” if  $\frac{\langle N_G \rangle}{N_p} > \frac{6}{10}$  and phase-separated otherwise,
2. “spongy mono-cluster” if phase-separated and if  $\langle n_{\text{coh}} \rangle_C / L_C N_p \geq \frac{13}{20}$  and if  $\langle R_g \rangle_C / \langle R_g \rangle_G \geq \frac{1}{4}$ ,
3. “mono-cluster” if phase-separated and if  $\langle R_g \rangle_C / \langle R_g \rangle_G \geq \frac{3}{20}$  and if  $\langle n_{\text{coh}} \rangle_C / \langle n_{\text{coh}} \rangle_G \geq \frac{1}{10}$ ,
4. “poly-cluster” if phase-separated and if  $\langle d_C \rangle_G / r_{\text{coh}} \geq 3$  and if  $\langle n_{\text{coh}} \rangle_C / \langle n_{\text{coh}} \rangle_G < \frac{3}{20}$ ,
5. else “other phase-separated”.

**B. Charge-spacer polymers.** The following conditionals should be followed (executed) one-by-one in order to reproduce the phase diagram (see Figs. S3B and 2C):

1. “Polymer-gas” if  $\frac{\langle N_G \rangle}{N_p} > \frac{4}{10}$  and phase-separated otherwise,
2. “poly-cluster” if phase-separated and if  $\langle N_C \rangle_G > 3$  and if  $\langle d_C \rangle_G / r_{\text{coh}} \geq 2$  and if  $\langle n_{\text{coh}} \rangle_C / \langle n_{\text{coh}} \rangle_G < \frac{7}{20}$ ,
3. “percolated network” if phase-separated and if  $\langle n_{\text{coh}} \rangle_C / L_C N_p \leq \frac{1}{10}$ ,
4. “mono-cluster” if  $\langle R_g \rangle_C / \langle R_g \rangle_G \geq \frac{1}{2}$  and if  $\langle n_{\text{coh}} \rangle_C / \langle n_{\text{coh}} \rangle_G \geq \frac{4}{10}$ ,
5. else “other phase-separated”.

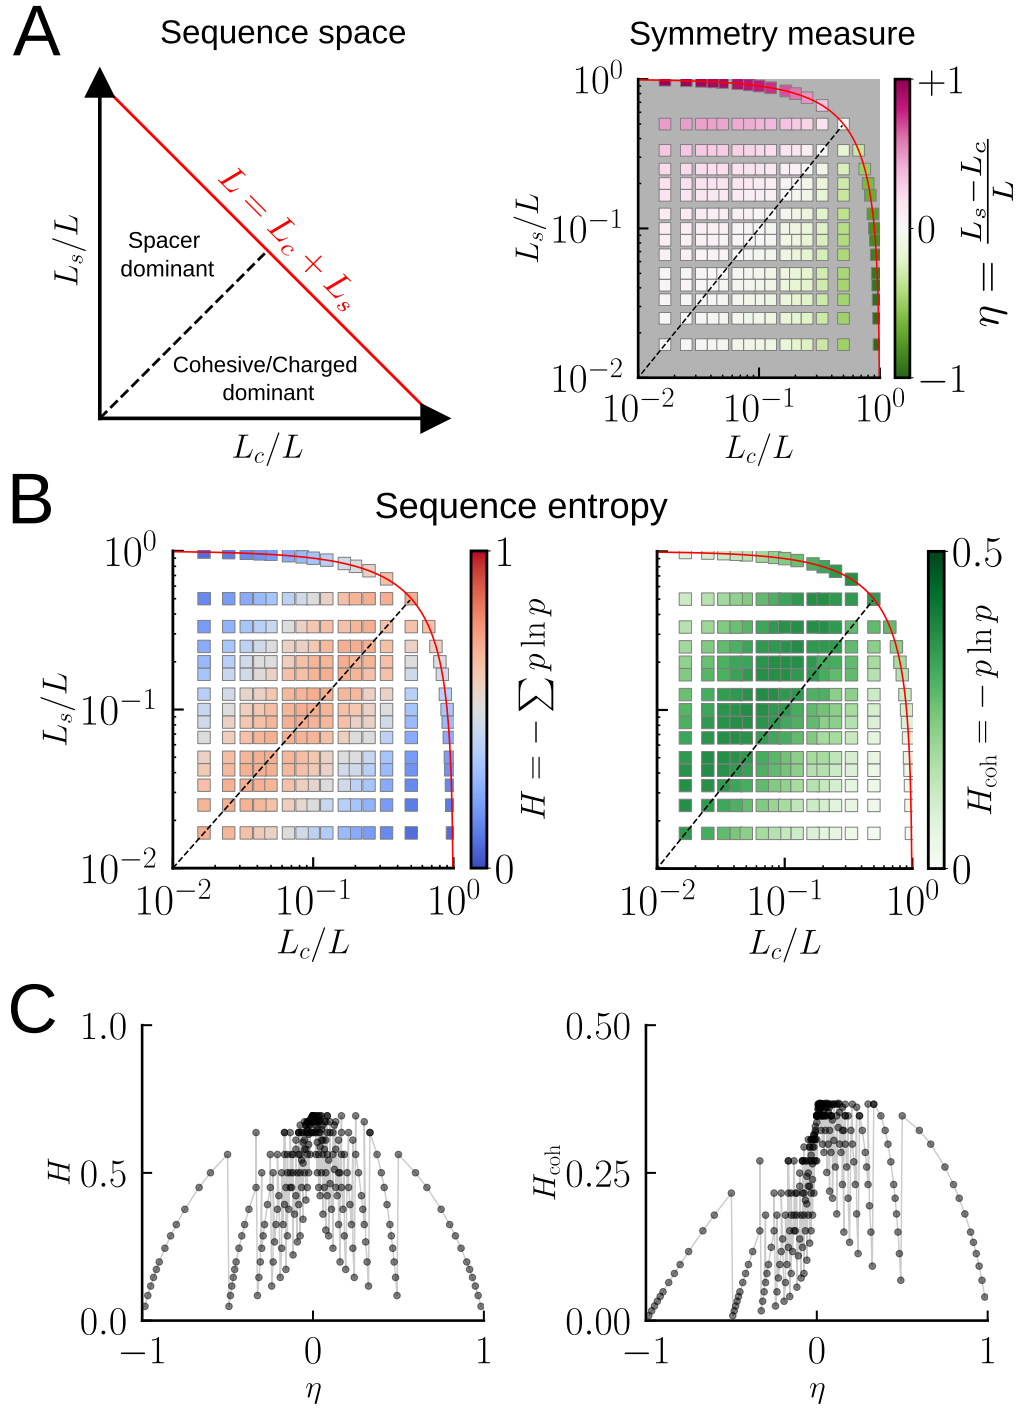

**Fig. S1.** (A) (Left) The space of all sequences defined by coordinate axes  $(L_s/L, L_c/L)$ , where  $L$  is the total number of beads in a chain. (Right) The symmetry measure quantifies the (im)balance between spacer and cohesive/charged block sizes. (B) (Left) The total Shannon entropy of the sequences. (Right) The Shannon entropy of the sequence, accounting only for the cohesives in the sequence. (C) (Left) Total Shannon entropy  $H$  against symmetry measure  $\eta$  and (right) Cohesive Shannon entropy  $H_{\text{coh}}$  against symmetry measure. Note that here, the total alphabet size was restricted to 2 where any bead in the  $L_c$  block is one character and any bead in the  $L_s$  block is another. Thus, cohesive-spacer and charge-spacer sequences with the same  $(L_c, L_s)$  will give the same Shannon entropy.

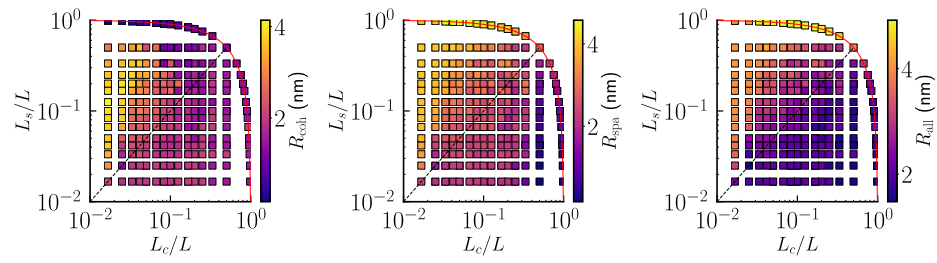

**Fig. S2. Single-polymer size metrics in a condensate context.** Averaged radius of gyration, per polymer, of the cohesives  $R_{\text{coh}}$  (left), spacers  $R_{\text{spa}}$  (centre), and all beads  $R_{\text{all}}$  (right) as a function of the sequence coordinates.

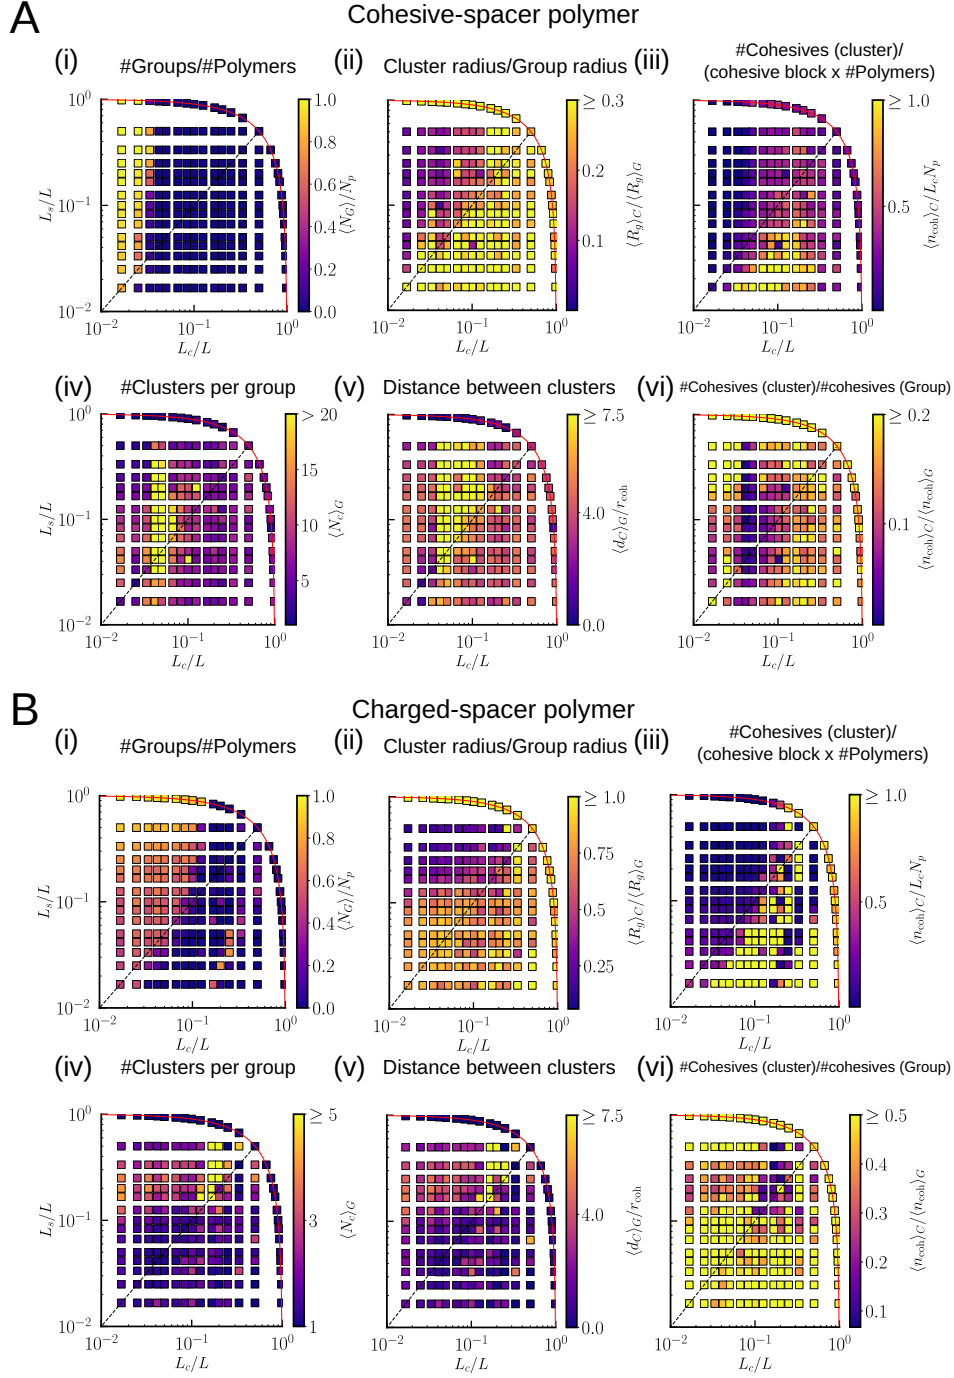

**Fig. S3. Quantification of many-polymer simulations.** (A) Quantification of cohesive-spacer polymer simulations for  $N_p = 100$  polymers: (i)  $\frac{\langle N_G \rangle}{N_p}$  is the averaged number of groups divided by the number of polymers, (ii)  $\frac{\langle R_g \rangle_C}{\langle R_g \rangle_G}$  is the averaged radius-of-gyration of the clusters divided by the averaged radius-of-gyration of the group, (iii)  $\frac{\langle n_{coh} \rangle_C}{L_C N_p}$  is the averaged number of cohesives per cluster divided by the cohesive block length multiplied by the number of polymers, (iv)  $\langle N_c \rangle_G$  is the averaged number of clusters per group, (v)  $\frac{\langle d_C \rangle_G}{r_{coh}}$  is the averaged distance between clusters per group divided by the cohesive interaction range, (vi)  $\frac{\langle n_{coh} \rangle_C}{\langle n_{coh} \rangle_G}$  is the averaged number of cohesives per cluster divided by the averaged number of cohesives per group. (B) The same as (A) but for the charge-polymer simulations.

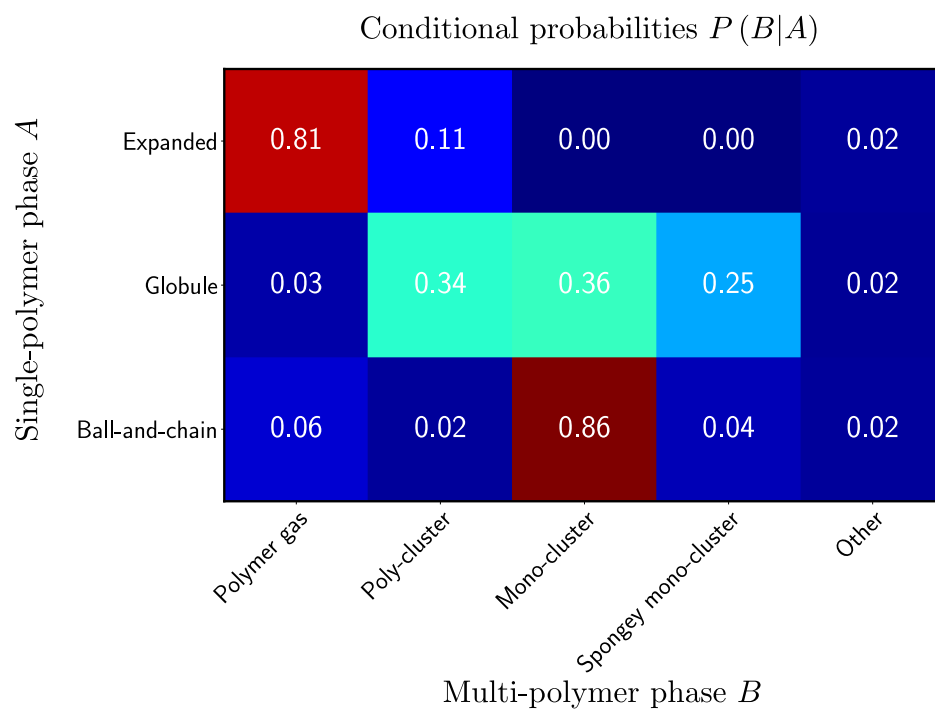

**Fig. S4. Single-polymer phases predict multi-polymer phase.** Conditional probabilities  $P(B|A)$  for a multi-polymer phase  $B$  given a single-polymer phase  $A$ . Here  $P(B|A) = P(B \cap A)/P(A)$ .

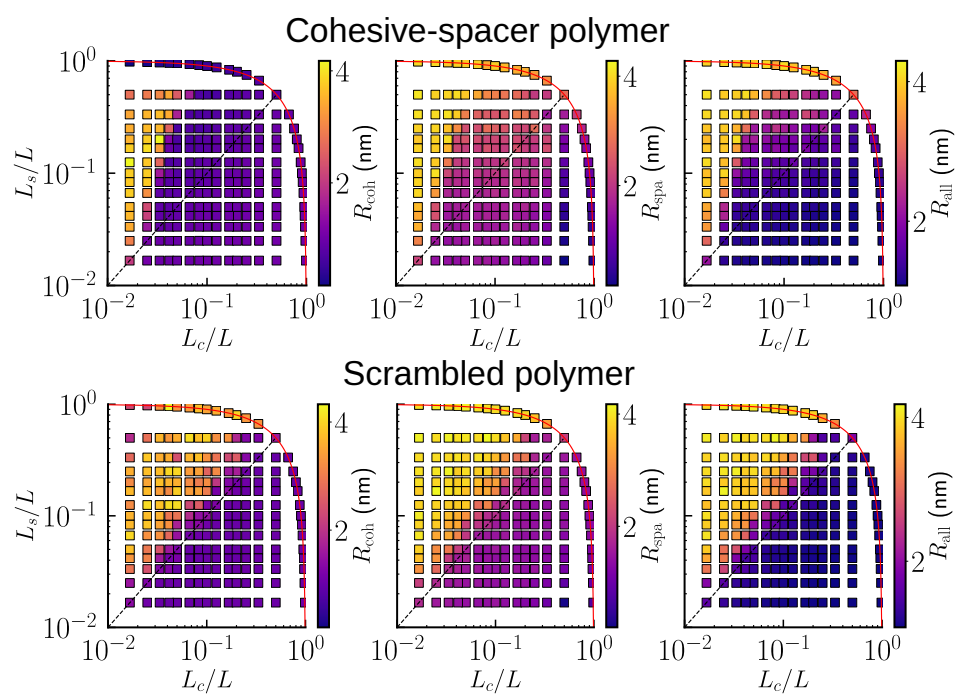

**Fig. S5. Scrambling homogenizes the behaviour of single polymers.** Averaged radius of gyration, per polymer, of the cohesives  $R_{\text{coh}}$ , spacers  $R_{\text{spa}}$ , and all beads  $R_{\text{all}}$  as a function of the sequence coordinates  $(L_c/L, L_s/L)$  for cohesive-spacer polymers (top) and scrambled cohesive-spacer polymers (bottom).
